# Supplementary material for: Surface Termination and Band Alignment in 2D Heterostructures
Source: arXiv:2408.05915 source file (2024-08-12)
Supplement: Supplementary file 1 [file SI_Type2_TMD.pdf]

# Supporting Information for Surface Termination and Band Alignment in 2D Heterostructures

Raheel Hammad<sup>\*,1</sup>, Snehith Adabala<sup>1</sup> and Soumya Ghosh<sup>\*,1</sup>

Tata Institute of Fundamental Research Hyderabad, Hyderabad-500046, Telangana, India.

E-mail: [raheelhammad@tifrh.res.in](mailto:raheelhammad@tifrh.res.in); [soumya.ghosh@tifrh.res.in](mailto:soumya.ghosh@tifrh.res.in)

This SI contains :

- Structure of supercell used for computing macroscopic average of  $b$ -MoO<sub>3</sub>
- Tables regarding band-offset data for  $2I$ -MoS<sub>2</sub>/ $b$ -MoO<sub>3</sub> and  $2I$ -MoS<sub>2</sub>/ $uL$ - $b$ -MoO<sub>3</sub>
- Schematic representation of band-offset corresponding to  $2I$ -MoS<sub>2</sub>/ $uL$ - $b$ -MoO<sub>3</sub>
- Structure of bulk unit cells for normal and alternate( $uL$ ) layering in PbCN<sub>2</sub>, CuSbS<sub>2</sub>, and TeO<sub>2</sub>
- Schematic representation of their corresponding band edges
- Additional details regarding equation 1 (main text) and generation of the heterostructures reported in the main text

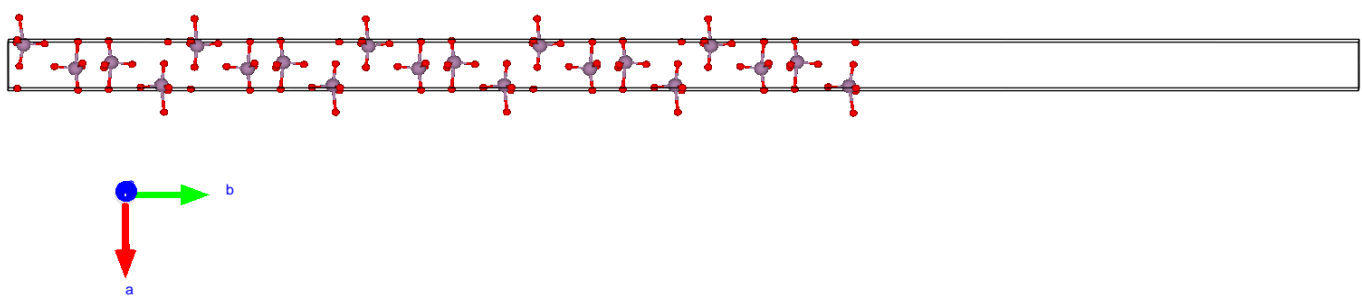

**Figure S1:** Supercell of MoO<sub>3</sub> required to compute the macroscopic average of bulk wrt to vacuum.

**Table-S1:** Band-offset data for 2I-MoS<sub>2</sub> /b-MoO<sub>3</sub>. The first column specifies the functional used for computing  $E_g$  and  $\bar{E}_i^{VBM}$ , respectively.  $e\bar{V}_{H,Vac}$  was computed using PBE functional only. The difference between  $\bar{E}_i^{VBM}$  and  $e\bar{V}_{H,Vac}$  gives  $\bar{E}_{i,vac}^{VBM}$ . VBO is computed from the difference in  $\bar{E}_{i,vac}^{VBM}$  of 2I-MoS<sub>2</sub> and b-MoO<sub>3</sub>.

| Setup        | $E_g$ (eV)  | $\bar{E}_i^{VBM}$ (eV) | $e\bar{V}_{H,Vac}$ (eV) | $\bar{E}_{i,vac}^{VBM}$ (eV) | VBO (eV) |
|--------------|-------------|------------------------|-------------------------|------------------------------|----------|
| PBE, PBE     | 1.311/2.072 | -1.243/0.829           | 4.287/ 8.957            | -5.530/ -8.128               | 2.598    |
| HSE06, HSE06 | 1.860/2.947 | -1.652/-0.296          | 4.287/ 8.957            | -5.939/-9.253                | 3.314    |
| HSE06, PBE   | 1.860/2.947 | -1.243/0.829           | 4.287/ 8.957            | -5.530/-8.128                | 2.598    |

**Table-S2:** Band-offset data for 2I-MoS<sub>2</sub> and uL-b-MoO<sub>3</sub>. The first column specifies the functional used for computing  $E_g$  and  $\bar{E}_i^{VBM}$ , respectively.  $e\bar{V}_{H,Vac}$  was computed using PBE functional only. The difference between  $\bar{E}_i^{VBM}$  and  $e\bar{V}_{H,Vac}$  gives  $\bar{E}_{i,vac}^{VBM}$ . VBO is computed from the difference in  $\bar{E}_{i,vac}^{VBM}$  of 2I-MoS<sub>2</sub> and b-MoO<sub>3</sub>.

| Setup        | $E_g$ (eV)  | $\bar{E}_i^{VBM}$ (eV) | $e\bar{V}_{H,Vac}$ (eV) | $\bar{E}_{i,vac}^{VBM}$ (eV) | VBO (eV) |
|--------------|-------------|------------------------|-------------------------|------------------------------|----------|
| PBE, PBE     | 1.311/2.072 | -1.243/0.829           | 4.287/7.755             | -5.530/-6.927                | 1.396    |
| HSE06, HSE06 | 1.860/2.947 | -1.652/-0.296          | 4.287/7.755             | -5.936 /-7.898               | 1.962    |
| HSE06, PBE   | 1.860/2.947 | -1.243/0.829           | 4.287/7.755             | -5.530/-6.927                | 1.396    |

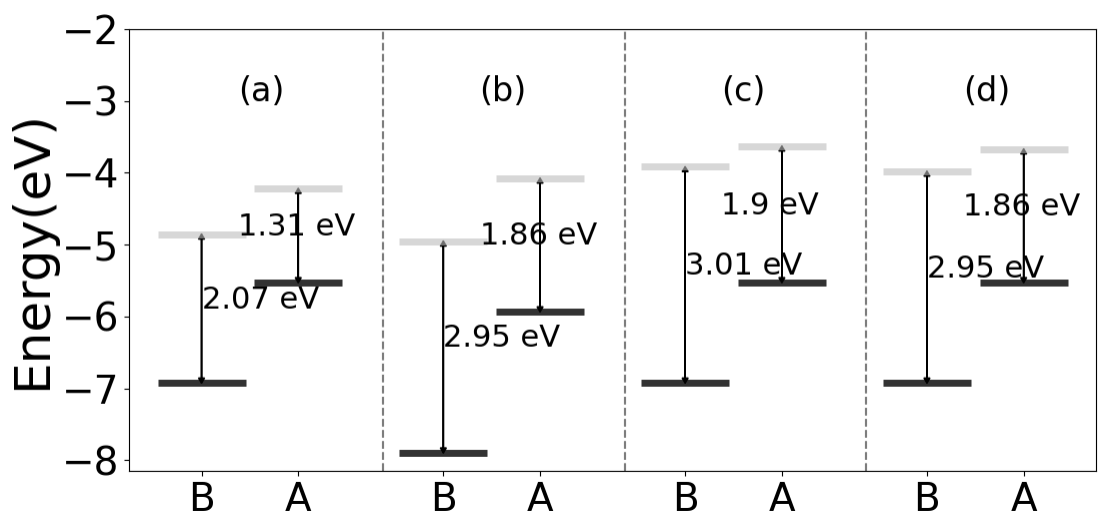

**Figure S2:** Band alignment between 2l-MoS<sub>2</sub>(**A**) and uL-*b*-MoO<sub>3</sub>(**B**) with different protocols to compute the VBOs and band gaps ( $E_g$ s). (a) Both VBOs and  $E_g$ s are computed with PBE (b) VBMs and  $E_g$ s are computed with HSE06 but the macroscopic averaging employing slabs is performed with PBE (c) VBOs are computed with PBE but  $E_g$ s are obtained from previously reported experimental data on isolated MoS<sub>2</sub> (layered) <sup>1</sup> and MoO<sub>3</sub> (bulk) <sup>2</sup> (d) VBOs are computed with PBE but  $E_g$ s are estimated with HSE06

### Extension to different systems.

Figure S3 shows the conventional (lower surface energy) and unconventional structures of PbCN<sub>2</sub>, CuSbS<sub>2</sub>, and TeO<sub>2</sub> respectively. These are just a few examples for demonstration purposes but there can be many more such layered materials where the aforementioned scheme can be applicable.

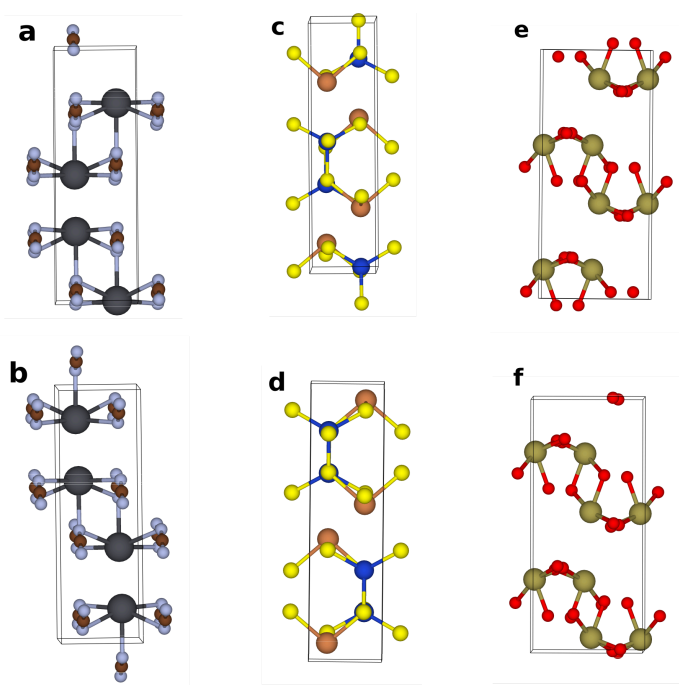

**Figure S3:** Conventional (a,c,e) and Unconventional(b,d,f) structures of  $\text{PbCN}_2$ ,  $\text{CuSbS}_2$  and  $\text{TeO}_2$  respectively

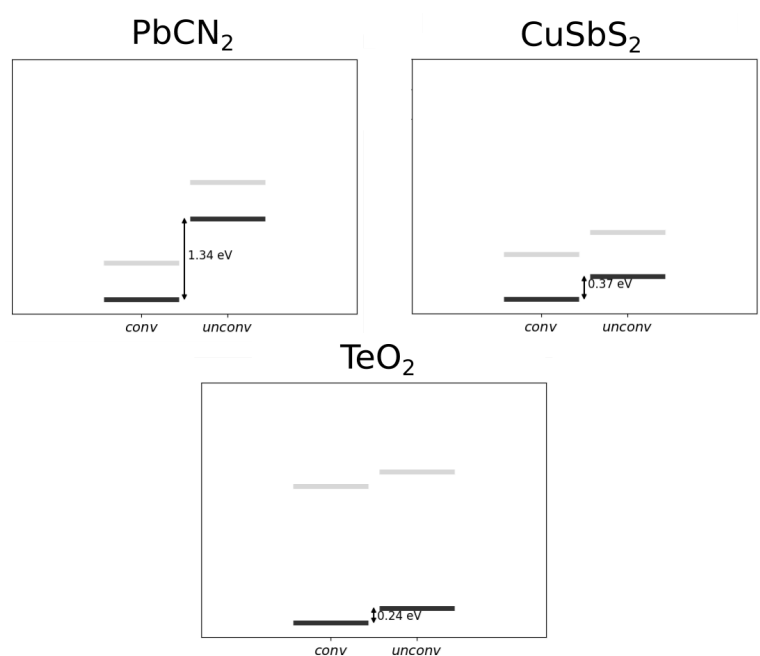

**Figure S4.** Shift in band-edges of the materials depending on how the layers are cleaved.

## Methods

Details regarding equation 1 in the main text.

$$\begin{aligned} E_{l-\text{MoS}_2/\text{vac}}^{\text{VBM}} &= E_{l-\text{MoS}_2}^{\text{VBM}} - E_{\text{vac}/l-\text{MoS}_2} \\ &= E_{l-\text{MoS}_2}^{\text{VBM}} - e\bar{V}_{\text{H},l-\text{MoS}_2} + e\bar{V}_{\text{H},l-\text{MoS}_2} - E_{\text{vac}/l-\text{MoS}_2} \\ &= \bar{E}_{l-\text{MoS}_2}^{\text{VBM}} - e\bar{V}_{\text{H},\text{vac}/l-\text{MoS}_2} \\ E_{b-\text{MoO}_3/\text{vac}}^{\text{VBM}} &= \bar{E}_{b-\text{MoO}_3}^{\text{VBM}} + e\bar{V}_{\text{H},b-\text{MoO}_3} - E_{\text{vac}/b-\text{MoO}_3} \\ &= \bar{E}_{b-\text{MoO}_3}^{\text{VBM}} - e\bar{V}_{\text{H},\text{vac}/b-\text{MoO}_3} \\ &\approx \bar{E}_{b-\text{MoO}_3}^{\text{VBM}} - e\bar{V}_{\text{H},\text{vac}/l-\text{MoO}_3} \end{aligned}$$

## Heterostructure details

### MoO<sub>3</sub>/MoS<sub>2</sub>

To make a heterostructure of MoS<sub>2</sub> and MoO<sub>3</sub> we require several individual units to minimize the lattice strain. A supercell of MoO<sub>3</sub> [4x3] with 15.849(Å) x 11.091(Å) is combined with an orthorhombic supercell of MoS<sub>2</sub>[5x2] with 15.908(Å) x 11.093(Å). Hence, the MoS<sub>2</sub> structure is subjected to lattice strain. Therefore in this case, there will be minimal strain in the 'a' and 'b' directions of 0.370% and 0.018% respectively. The heterostructures are geometry-optimized before any electronic structure calculations.

### MoO<sub>3</sub>/MoTe<sub>2</sub>

A supercell of MoO<sub>3</sub> [3x1] 11.887 (Å) x 3.697 (Å) is combined with an orthorhombic supercell of MoTe<sub>2</sub>[5x2] 12.28 (Å) x 3.547 (Å). For the heterostructure we have used the lattice parameters of MoO<sub>3</sub>, hence there will be strain of 3.2 % and 4.22% on MoTe<sub>2</sub> in the 'a' and 'b' lattice direction. The heterostructure is then allowed to relax before proceeding with the electronic structure calculations.

## **CuSbS<sub>2</sub>/CdS**

Supercell of CuSbS<sub>2</sub> [2x2] with 7.603 (Å) x 12.146 (Å) is combined with an orthorhombic supercell of CdS [2x3] with 7.480 (Å) x 12.946 (Å). For the heterostructure we have used the lattice parameters of CuSbS<sub>2</sub>, hence there will be strain of 1.6% and 6% on CdS in the 'a' and 'b' direction respectively.

## References

- (1) Ganatra, R.; Zhang, Q. Few-layer MoS<sub>2</sub>: a promising layered semiconductor. ACS nano2014, 8, 4074–4099.
- (2) Chen, Y.; Lu, C.; Xu, L.; Ma, Y.; Hou, W.; Zhu, J.-J. Single-crystalline orthorhombic molybdenum oxide nanobelts: synthesis and photocatalytic properties. CrystEngComm 2010, 12, 3740–3747
